# Supplementary material for: Engineering two-dimensional kagome topological insulator from porous graphene
Source: arXiv:2412.11516 source file (2024-12-16)
Supplement: Supplementary file 1 [file supp.pdf]

**Supplementary Material for**

# Engineering a two-dimensional kagome topological insulator from porous graphene

Shashikant Kumar,[1] Gulshan Kumar,[1] Ajay Kumar,[1] and Prakash Parida[1, a)]

*Department of Physics, Indian Institute of Technology Patna, Bihta, Bihar, 801106, India*

[a)]Electronic mail: pparida@iitp.ac.in

## 1. COMPUTATIONAL DETAILS OF DENSITY FUNCTIONAL THEORY

Density functional theory (DFT) implemented within the Vienna ab initio simulation package (VASP) was used to investigate the electronic properties of PGKL. The simulations employed the projector augmented wave (PAW) approach, emphasizing interactions between valence and core electrons, and periodic boundary conditions. Boron, carbon, and nitrogen pseudo-potentials were used with electronic configurations of $2s^2 2p^1$, $2s^2 2p^2$, and $2s^2 2p^3$, respectively. All carbon-based kagome structures exhibited a rhombus unit cell with a periodic pattern in the x-y plane, and a vacuum of 20 Å was applied to prevent interactions along the z-axis. The Perdew–Burke–Ernzerhof (PBE) generalized-gradient approximation (GGA) was employed for the exchange-correlation potential. The plane wave energy cutoff value and k-mesh grid were 600 $eV$ and $11 \times 11 \times 1$, respectively. The conjugate-gradient approach was utilized for full crystal structure relaxation, with a force tolerance criterion set to $10^{-3}$ $eV/\text{Å}$ for each atom. Additionally, energy convergence criteria of $10^{-8}$ $eV$ were maintained throughout the calculation. Electronic band structures along high symmetry points $\Gamma - K - M - \Gamma$ in the first Brillouin zone were calculated.

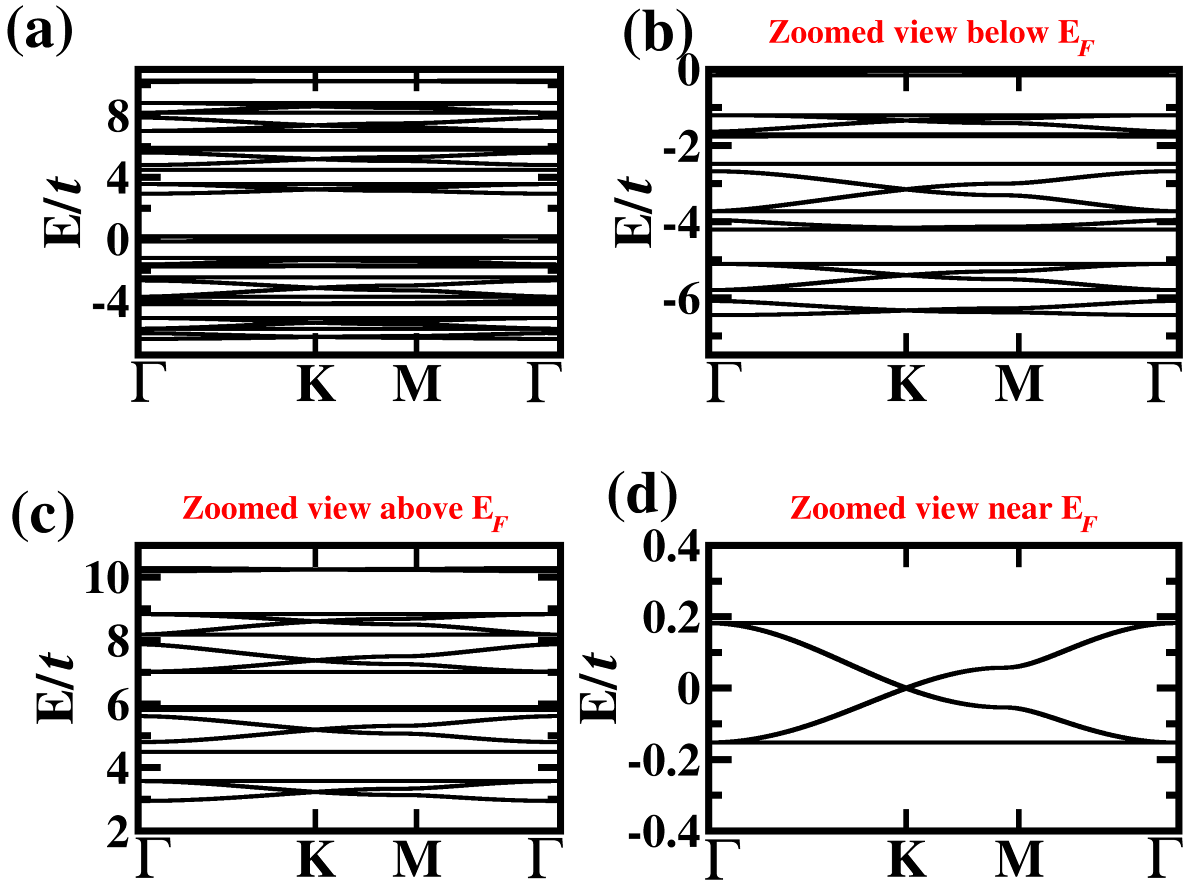


Fig S1. The TB electronic band structures of PGKL are depicted along the high-symmetry points in the Brillouin zone. Panel (a) illustrates the overall band structure of PGKL, while panels (b), (c), and (d) focus on the band structures below, above, and near the Fermi level, respectively.

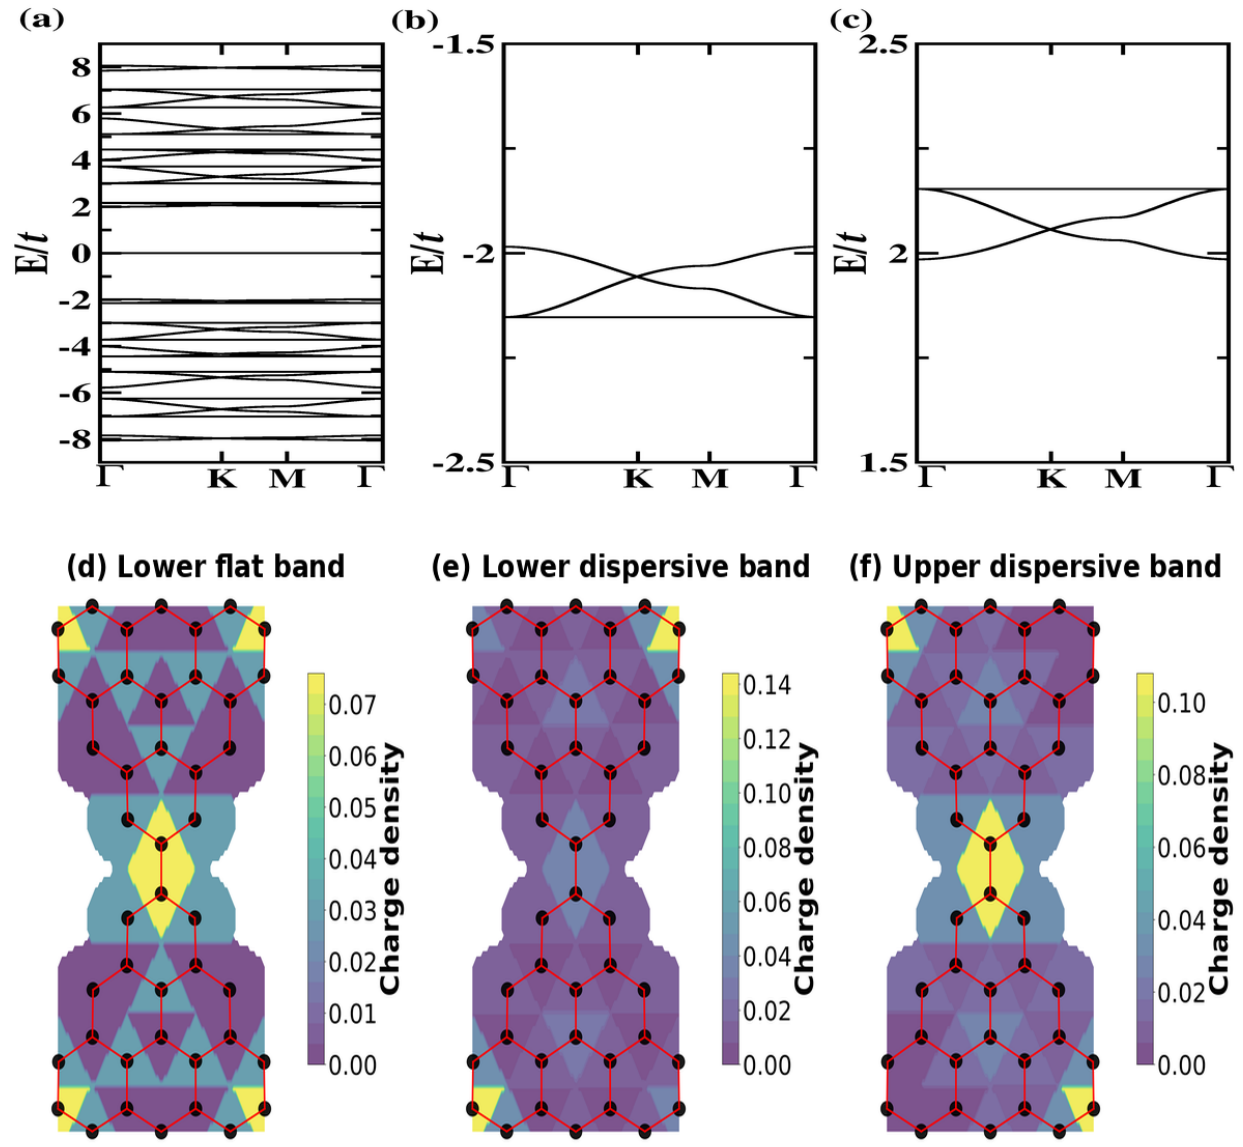


Fig S2. The TB electronic band structures of PGKL are depicted along the high-symmetry points in the Brillouin zone. Panel (a) illustrates the overall band structure of PGKL, while panels (b) and (c) focus on the band structures below and above the Fermi level, respectively. Panel (d) depicts the charge density of the flat band, while panels (e) and (f) depict the charge density of two dispersive bands present around E/t= -2 in the figure S2(b). The onsite energy for bulk and edge atoms are set to $\epsilon_{bulk} = 0$ eV, and $\epsilon_{edge} = 0$ eV.

## 2. EFFECTS OF PORE SIZE ON BAND WIDTH OF DIRAC BANDS NEAR THE FERMI LEVEL IN PGKL

From Fig. S3, we notice that, the band width (W) of the Dirac band reduces with increasing pore sizes (increasing the supercell size) without opening an energy-gap at the Fermi level. This trend may be attributed to two reasons: (i) the quantum confinement effect gets enhanced with increasing pore sizes, which in turn reduces the Fermi velocity and the band width of the Dirac bands near the Fermi level. Usually, a gap is expected in the energy spectrum because of the quantum confinement and localisation of electrons. However, interestingly, the honeycomb-kagome symmetry in PGKL structure prevents it from opening up a band-gap near the Fermi level. In Fig. S3 (b) to clearly show that, the bandwidth reduces exponentially with the supercell size (pore size) similar to the exponential reduction of the nearest neighbor hopping integral with the bond length[1,2]. (ii) While we have already cited a few references (37–43 in the main manuscript) where an energy-gap is opened up or flat-bands appear near the Fermi level for the porous graphene, our undoped porous graphene interestingly behaves like a gapless graphene with reduced band width of Dirac bands near the Fermi level. The emergence of Dirac bands in our uniquely designed porous structure is attributed to the inherent honeycomb arrangement of neighboring NNCT atoms. In Fig. S5, the separation between two nearest-neighbor NNCT atoms (marked as a ring) is 7 times the C-C bond length in pristine graphene ($C - C = b_0 = 1.42\,\text{Å}$), defined as $b = 7b_0 \approx 10\,\text{Å}$. These NNCT atoms form a honeycomb structure and interact with each other despite being separated by a large distance ($\approx 10\,\text{Å}$). This interaction results in the formation of a Dirac band near the Fermi level, similar to graphene. Interestingly, even though we do not include a direct hopping term between the NNCT atoms in our TB model, they still interact between them through carbon chains linking them, giving rise to the observed Dirac bands. This phenomenon highlights the presence of long-range interactions in the PGKL structure which may be expected in covalent organic framework (COF) types of structures. If valence electrons near the Fermi level exhibit such a long-range correlation, there is a high possibility of chemical synthesis of its extended sheet through bottom-up approach. Remarkably, this long-range interaction showing Dirac bands has been experimentally observed using ARPES in similar 2D structures, where only a few selective edge groups (our case $-$CH) are different, e.g., $-\mathrm{C} = O$, $-$O, and $-CH_2$ groups[3–5].

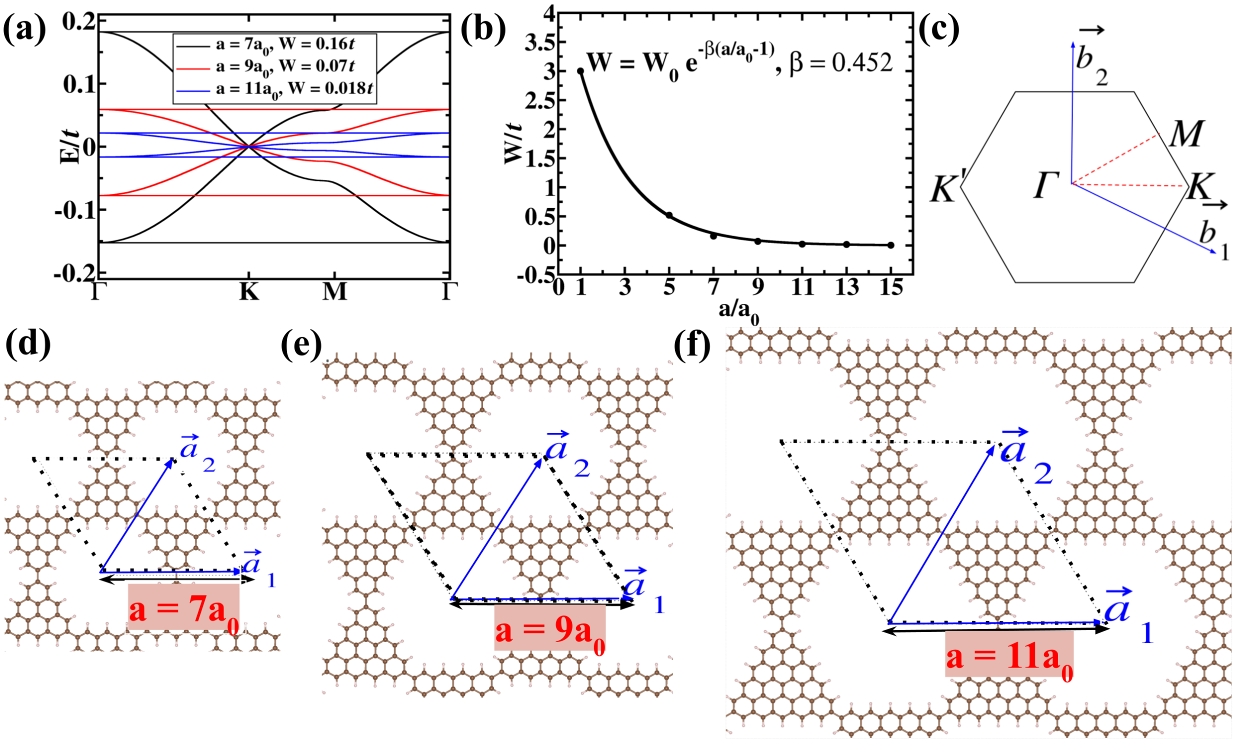


Fig S3. (a) illustrates the band structure near the Fermi level for different supercell sizes, where "W" denotes the band-width of the Dirac bands in PGKL. (b) The dependence of the normalized band width $\frac{W}{W_0}$ on the lattice constant $a$ in PGKL, fitted with an exponential decay. $a_0 = 2.46\mathring{A}$ is the lattice constant in pristine graphene and $W_0 = 3t$ is the bandwidth of pristine graphene. (c) shows the first Brillouin zone of the PGKL lattice, with high-symmetry points ($\Gamma$, $K$, and $M$) and the reciprocal lattice vectors $\vec{b}_1$ and $\vec{b}_2$. A few represents structures are given in panels (d), (e), and (f) for $a = 7a_0$, $a = 9a_0$, and $a = 11a_0$. The black dotted lines outline rhombic unit cell in each structure. The lattice structure is represented by the primitive vectors $\vec{a}_1 = a(1,0)$ and $\vec{a}_2 = a\left(\frac{1}{2}, \frac{\sqrt{3}}{2}\right)$. In reciprocal space, the corresponding lattice vectors are $\vec{b}_1 = \left(\frac{2\pi}{a}, -\frac{2\pi}{\sqrt{3}a}\right)$ and $\vec{b}_2 = \left(0, \frac{4\pi}{\sqrt{3}a}\right)$. High-symmetry points within the Brillouin zone include the $\Gamma$ point at $(0,0)$, the $K$ point at $\left(\frac{4\pi}{3a}, 0\right)$, and the $M$ point at $\left(\frac{\pi}{a}, \frac{\pi}{\sqrt{3}a}\right)$.

## 3. BAND STRUCTURES AND CHARGE DENSITY PLOTS FOR VARIOUS CASES

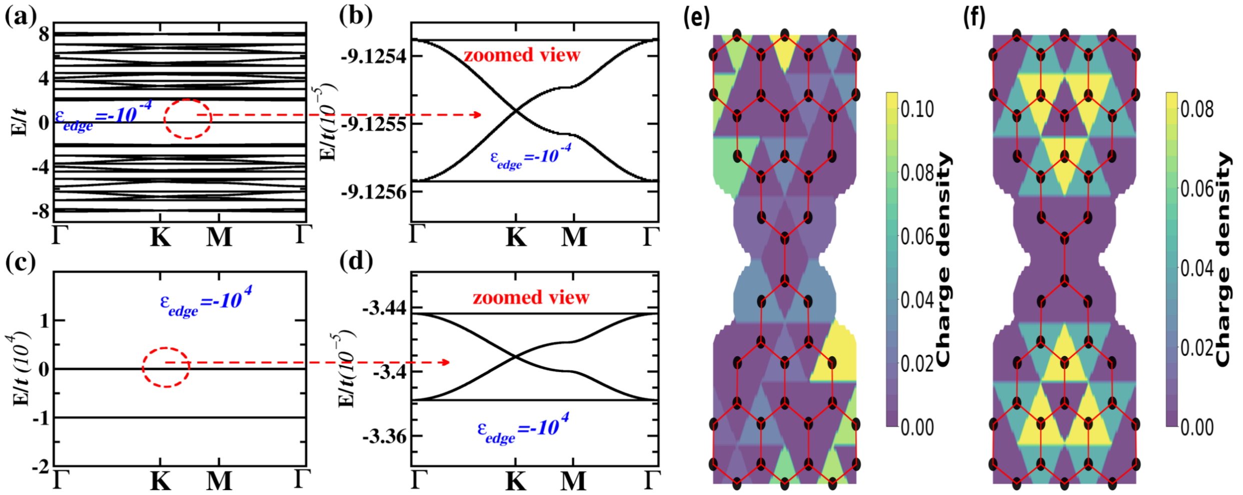


Fig S4. The TB band structures of PGKL are plotted along the high-symmetry points. Panels (a) and (b) represent the band structures where the onsite energy of the edge atoms is set to $\epsilon_{\text{edge}} = -10^{-4}$ eV. Panels (c) and (d) show the band structures where the onsite energy of the edge atoms is set to $\epsilon_{\text{edge}} = -10^{4}$ eV. Panels (e) and (f) present the charge density near the Fermi level for one of the four flat bands correspond (a) and (c), respectively. The charge density plots for three other flat bands are very similar to this.

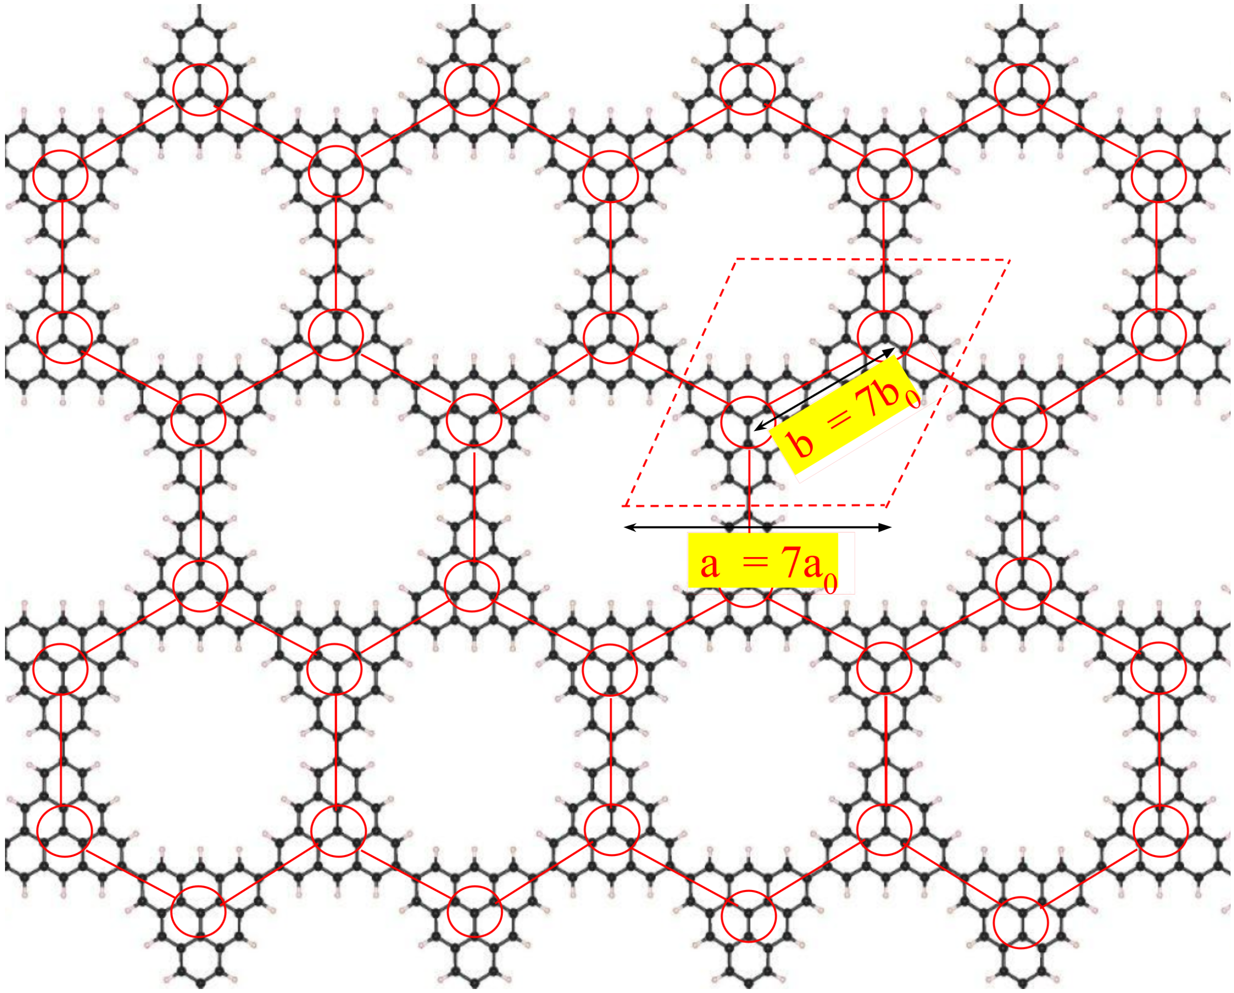


Fig S5. Schematic representation of PGKL, where the red solid lines depict the periodic honeycomb lattice, red circles mark the nearest neighbors of the centroid atom within the triangle, and the red dashed lines outline its unit cell. The separation between two nearest neighbor NNCT atoms (ring) is 7 times of C-C bond length in graphene ($b_0 = 1.42\mathring{A}$), is defined as $b = 7b_0 \approx 10\mathring{A}$, whereas lattice constant $a_0 = \sqrt{3}b_0$.

## 4. DOPING THE CENTROID ATOMS WITH BORON OR NITROGEN

In PGKL structure, the centroid of a triangle of atoms are doped with boron or nitrogen atoms, the resulting band structure is illustrated in Fig. S6. We set onsite energy of B and N atoms to 1.59 eV and -1.59 eV, respectively. The shift in Fermi level from the Dirac band to the flat band occurs when the central atom of the triangle (carbon) is replaced by boron or nitrogen. Boron has one fewer electron than carbon, while nitrogen has one more electron than carbon. In the PGKL structure, within the unit cell, two carbon atoms are replaced

by either nitrogen or boron. In a half-filled scenario, this replacement causes one band to be either less filled or more filled up to the Fermi level. In our study, we observe two flat bands and two Dirac bands, with the Dirac bands situated between the flat bands. In the undoped case, the Fermi level lies in the middle of the two Dirac bands. However, doping with boron or nitrogen results in a shift of the Fermi level either upwards or downwards. Specifically, the Fermi level moves upward or downward depending on the dopant, which reflects the electron deficiency or surplus introduced by boron or nitrogen, respectively. Upon doping with B/N atoms, the band structure still maintains a semi-metallic nature, with the Fermi level shifting from the Dirac point to near the flat band. Although doping occurs at the CT atoms, except a shift of the Fermi level, the effect of doping is not pronounced on the over all nature of those four low energy bands because of no significant contribution from the centroid atoms to those bands. However, NNCT atoms majorly contribute to those bands and hence any doping at the CT atoms has no impact on those bands. Upon including ISOC, a non-zero gap appears, accompanied by a non-zero spin Chern number below the gap. The transition from semi-metallic to insulator is evident, as illustrated in Fig. S7.

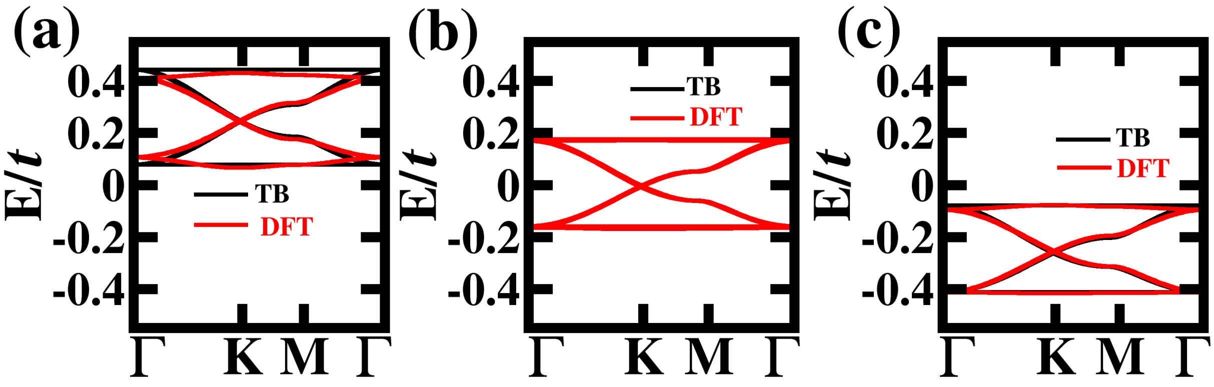


Fig S6. The TB and DFT band structures of PGKL are plotted along the high-symmetry points in the Brillouin zone, focusing on the vicinity of the Fermi level. Panels (a), (b), and (c) correspond to the boron, carbon, and nitrogen atoms at the centroid of the triangle within the lattice, respectively. The DFT band structures are depicted in red, while the TB band structures are represented in black. The onsite energy for edge atoms is set to $\epsilon_{edge} = -3.55\ eV$. The onsite energy of the centroid atom of the triangle for boron and nitrogen atoms is set to $\epsilon_B = 1.59\ eV\ and\ \epsilon_N = -1.59\ eV$, respectively. The Fermi level is scaled to zero.

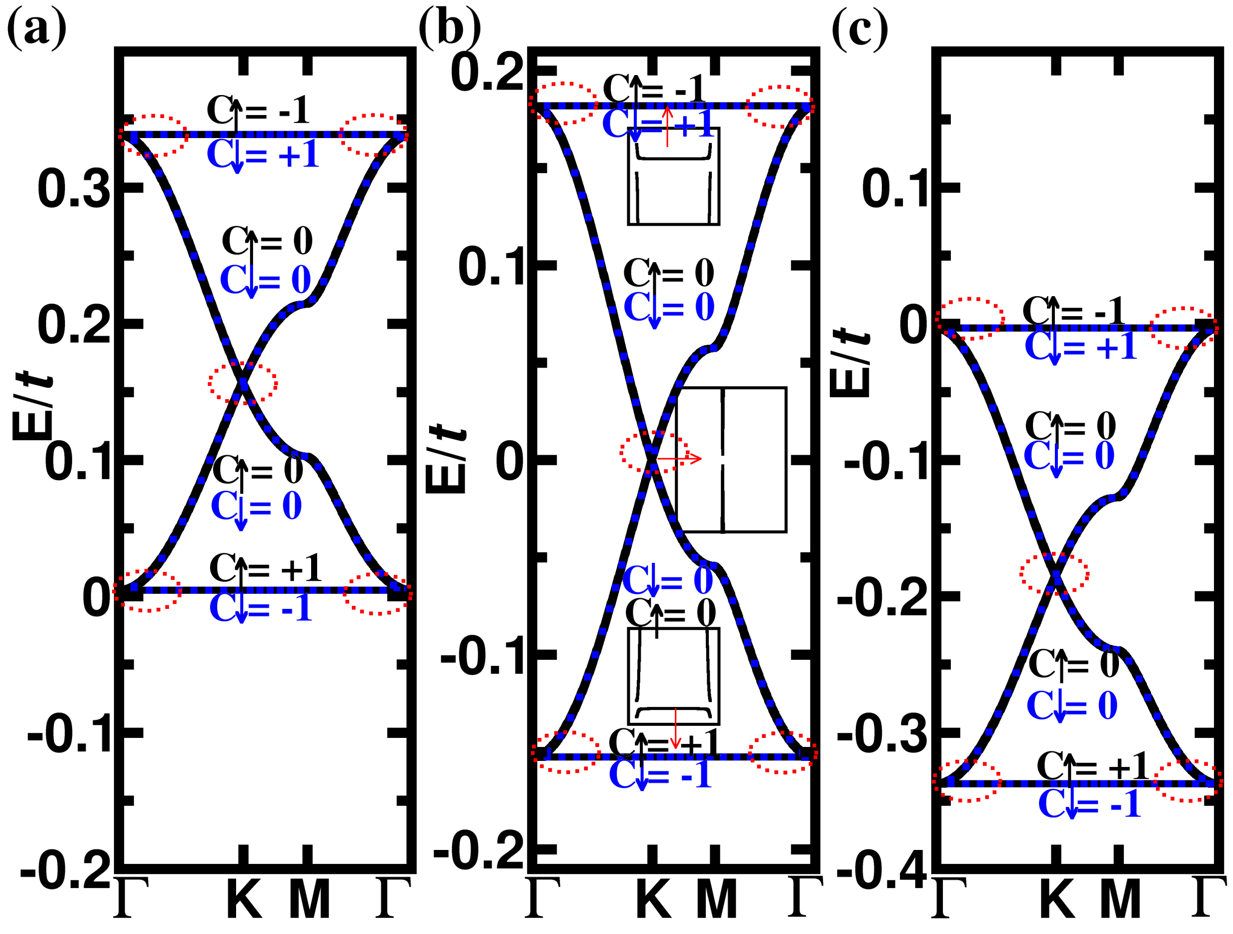


Fig S7. The TB band structure with ISOC for PGKL is plotted along the high-symmetry points in the Brillouin zone, focusing on the vicinity of the Fermi level. Panels (a), (b), and (c) correspond to the boron, carbon, and nitrogen atoms at the centroid of the triangle within the lattice, respectively. The onsite energy for each C atom at the edge is set to $\epsilon_{\text{edge}} = -3.55\ eV$. The onsite energy of the centroid atom of the triangle for boron and nitrogen atoms are set to $\epsilon_B = 1.59\ eV\ and\ \epsilon_N = -1.59\ eV$, respectively.

## 5. STUDY OF 1-D NANORIBBONS OF PGKL

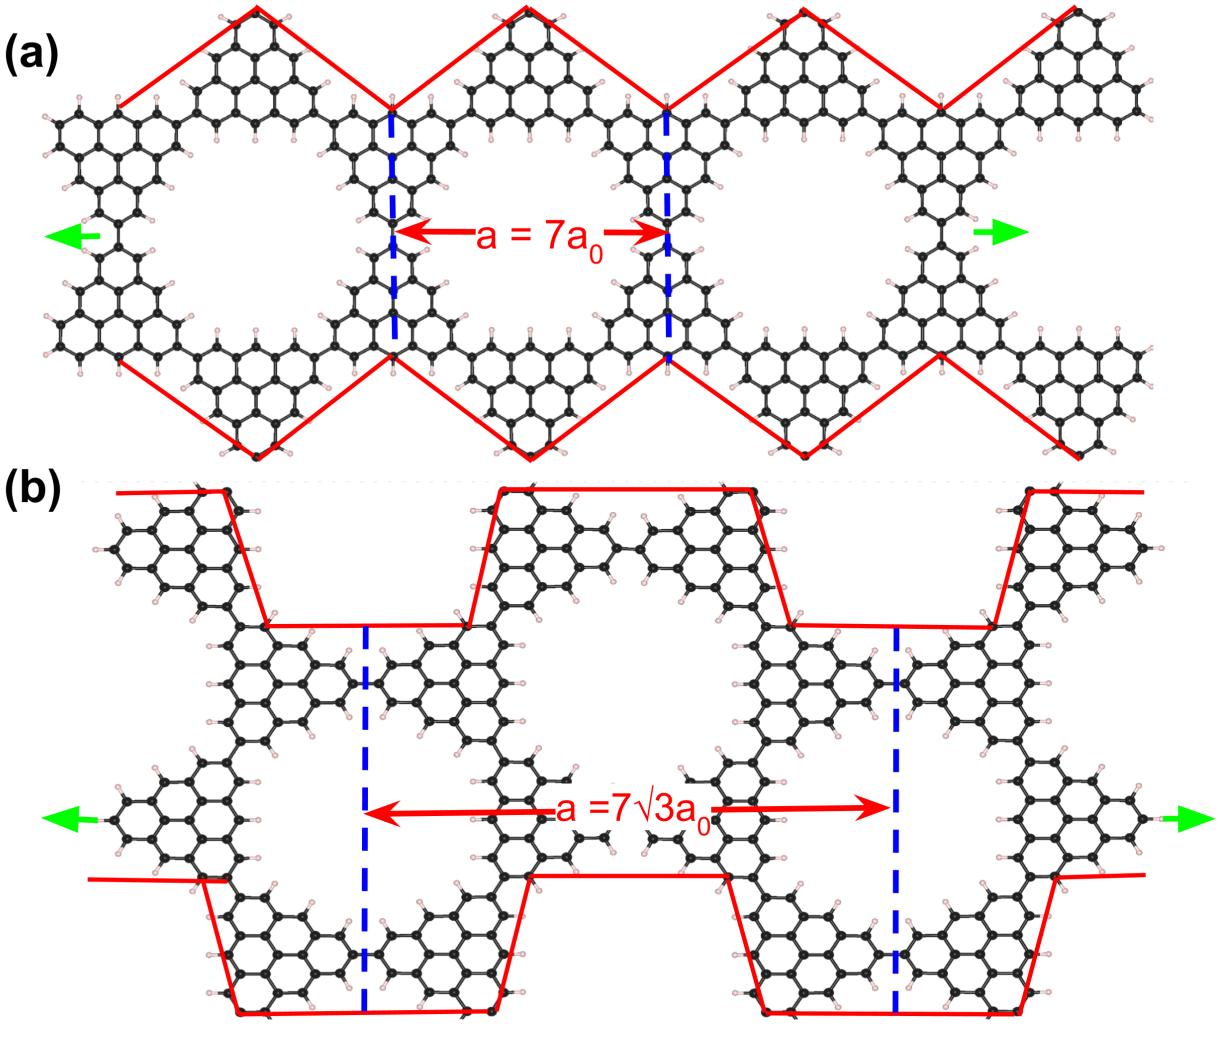


Fig S8. Schematic representations of PGKL are shown in panels (a) and (b), illustrating the structures of zigzag-like and armchair-like ribbons, respectively. The red line indicates the zigzag and armchair-like ribbons. The green arrow shows the periodic direction, while the blue dashed line represents the unit cell of the 1-D ribbon. For the zigzag ribbon, the lattice constant is $a = 7a_0$, while for the armchair ribbon, it is $a = 7\sqrt{3}a_0$.

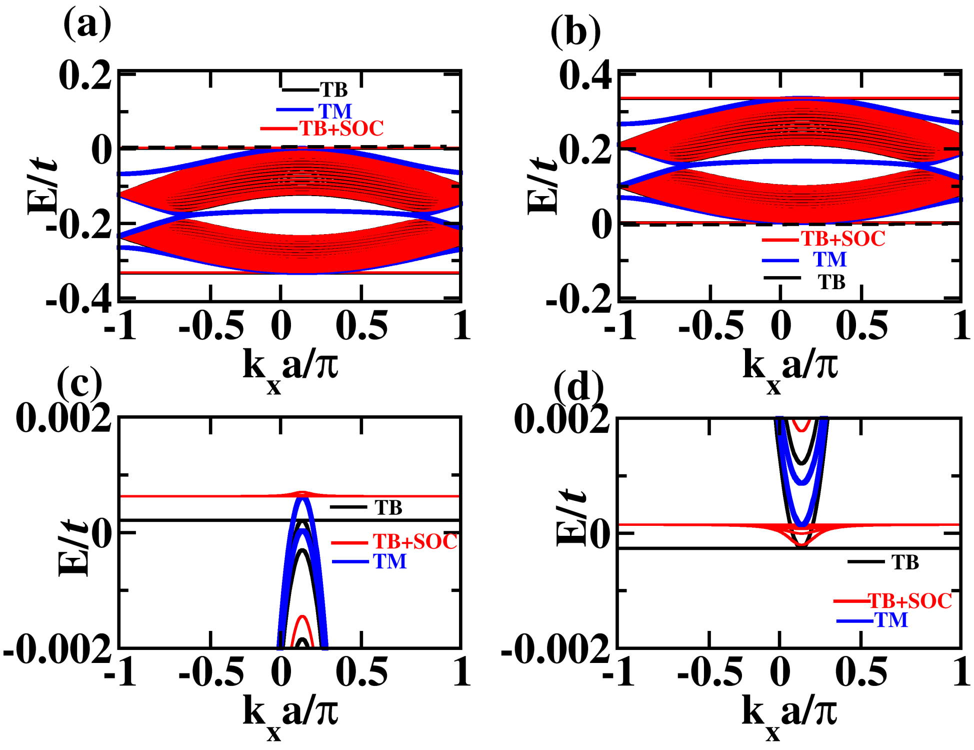


Fig S9. The band structure of (a) nitrogen and (b) boron doped 1-D zigzag PGKL. Panels (c) and (d) provide the zoomed-in view of (a) and (b), respectively. The black and red lines illustrate the band structures without and with ISOC, respectively. The blue line corresponds to the topological modes (TM), while the black dotted line indicates the Fermi level, which is scaled to zero.

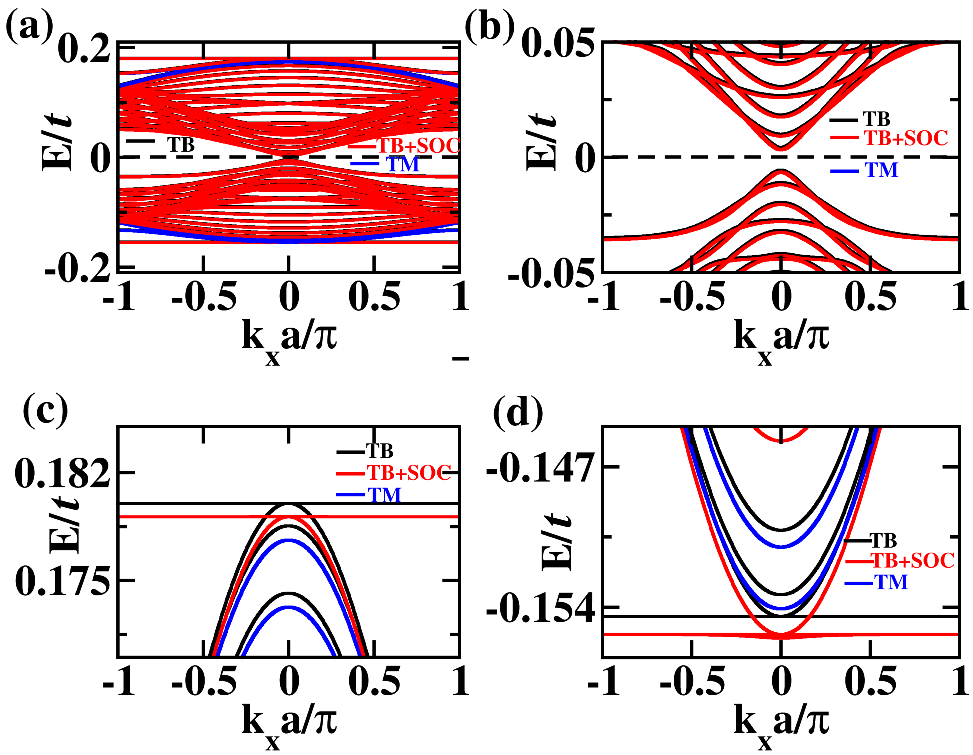


Fig S10. The band structure of the 1-D armchair-like ribbon of the PGKL is depicted, with panels (a), (b), (c), and (d) representing the regions near, at, above, and below the Fermi level, respectively. The black and red lines illustrate the band structures without and with ISOC, respectively. The blue line corresponds to the topological modes (TM), while the black dotted line indicates the Fermi level, which is scaled to zero.

## REFERENCES

[1]V. M. Pereira, A. Castro Neto, and N. Peres, "Tight-binding approach to uniaxial strain in graphene," Physical Review B—Condensed Matter and Materials Physics **80**, 045401 (2009).

[2]P. Li, J. Lu, W. Y. Wang, X. Sui, C. Zou, Y. Zhang, J. Wang, D. Lin, Z. Lu, H. Song, *et al.*, "Lattice distortion-enhanced superlubricity of (mo, x) s 2 (x= al, ti, cr and v) with moiré superlattice," Nanoscale **13**, 16234–16243 (2021).

[3]G. Galeotti, F. De Marchi, E. Hamzehpoor, O. MacLean, M. Rajeswara Rao, Y. Chen, L. Besteiro, D. Dettmann, L. Ferrari, F. Frezza, *et al.*, "Synthesis of mesoscale ordered two-dimensional $\pi$-conjugated polymers with semiconducting properties," Nature Materials **19**, 874–880 (2020).

[4]C. Steiner, J. Gebhardt, M. Ammon, Z. Yang, A. Heidenreich, N. Hammer, A. Görling, M. Kivala, and S. Maier, "Hierarchical on-surface synthesis and electronic structure of carbonyl-functionalized one-and two-dimensional covalent nanoarchitectures," Nature communications **8**, 14765 (2017).

[5]Y. Jing and T. Heine, "Two-dimensional kagome lattices made of hetero triangulenes are dirac semimetals or single-band semiconductors," Journal of the American Chemical Society **141**, 743–747 (2018).
